# Supplementary material for: Joint discrete and continuous matrix distribution modelling
Source: arXiv:2207.01364 source file (2022-07-04)
Supplement: Supplementary file 1 [file Appendix.tex]

\lstset{
    language=R,
    basicstyle=\scriptsize\ttfamily,
    commentstyle=\ttfamily\color{gray},
    numbers=left,
    numberstyle=\ttfamily\color{gray}\footnotesize,
    stepnumber=1,
    numbersep=5pt,
    backgroundcolor=\color{white},
    showspaces=false,
    showstringspaces=false,
    showtabs=false,
    frame=single,
    tabsize=2,
    captionpos=b,
    breaklines=true,
    breakatwhitespace=false,
    title={},
    escapeinside={},
    keywordstyle={},
    morekeywords={}
    }

\section*{Appendix}
In the following section all \texttt{R} code used in the report can be found
\lstinputlisting[caption=R code used in assignment]{Assignment3.R}
